# Supplementary material for: Tractable and Consistent Random Graph Models
Source: arXiv:1210.7375 source file (2014-06-25)
Supplement: Supplementary file 1 [file AppendixTable3.pdf]

| | | Data | Link-based model with covariates | Link-based model with extended covariates | SUGM with links and triangles | SUGM with isolates, links and triangles |
|---|---|---|---|---|---|---|
| | | [1] | [2] | [3] | [4] | [5] |
| Models are fit to different combinations of these statistics. | Number of Unsupported Links | 160.8 | 236.2 | 236.2 | 161.2 | 161.8 |
| | Number of Triangles | 39.2 | 3.1 | 3.1 | 39.7 | 39.5 |
| | Average Degree | 2.3243 | 2.3260 | 2.3234 | 2.5916 | 2.5219 |
| | Number of Isolates | 54.9722 | 25.7222 | 27.3750 | 31.4444 | 65.9167 |
| None of the models are directly fit to any of these statistics. | Average Clustering | 0.0895 | 0.0105 | 0.0134 | 0.1268 | 0.0829 |
| | Fraction in Giant Component | 0.7061 | 0.8315 | 0.8082 | 0.7982 | 0.6718 |
| | First Eigenvalue | 5.5446 | 3.8578 | 4.0746 | 4.6762 | 5.3025 |
| | Spectral Gap | 0.9550 | 0.3354 | 0.3728 | 0.6684 | 1.0617 |
| | Second Eigenvalue of Stochastized Matrix | 0.9573 | 0.9632 | 0.9642 | 0.9559 | 0.9069 |
| | Average Path Length | 4.6921 | 5.6565 | 5.5407 | 5.1215 | 4.1180 |

Notes: Column [1] presents the average value of various network characteristics across the 36 villages. Columns [2], [3], [4] and [5] present simulation results. In a simulation we first estimate parameters of a given model for a given village and then randomly draw a graph from the model with the estimated parameters. We run 100 simulations for each of the villages for each of the models and average across the simulations, and the entries report these averaged across the villages.
